# Supplementary material for: Optimality of intercellular signaling: direct transport versus diffusion
Source: arXiv:2204.09768 source file (2022-10-24)
Supplement: Supplementary file 1 [file supp_R2.pdf]

# Supplementary Material for
# Optimality of intercellular signaling: direct transport versus diffusion

Hyunjoong Kim,[1,*] Yoichiro Mori,[1,2] and Joshua B. Plotkin[1,2]

[1] *Center for Mathematical Biology & Department of Mathematics, University of Pennsylvania, Philadelphia, PA 19104, USA*

[2] *Department of Biology, University of Pennsylvania, Philadelphia, PA 19104, USA*

(Dated: October 12, 2022)

## S1. SINGLE PROTRUSION EVENT WITH IDEALIZED TARGETS

In this section, we present the computation for the hitting probability and the conditional mean protrusion lengths in two idealized targets.

### A. Disk-shaped target

In terms of target parameters, the target distance function is

$$\zeta(\Theta) = (r+d)\cos\Theta - \sqrt{r^2 - (r+d)^2\sin^2\Theta}, \quad \text{(S1.1)}$$

for $\Theta \in \phi(\Omega)$. Then the cumulative density function (cdf) of EPL can be written by

$$F_Z(x) = \int_{\zeta(y)\le x} \rho_\Theta(y)dy, \quad \text{(S1.2)}$$

which yields

$$F_Z(x) = \frac{1}{\sigma}\begin{cases} 0, & x \le d \\ \min\{\zeta^{-1}(x), \phi_{\max}, \sigma\}, & x > d \end{cases}. \quad \text{(S1.3)}$$

Here $\phi_{\max} = \max\{\phi(\Omega)\} = \sin^{-1}(r/(r+d))$. Then the hitting probability satisfies

$$\rho_{\mathrm{DT}} = \int_0^\infty \rho_L(x)F_Z(x)dx.$$

Performing integration yields

$$\rho_{\mathrm{DT}} = \frac{1}{\sigma}\int_0^{\sigma_0} e^{-\zeta(y)/l}dy, \quad \text{(S1.4)}$$

where $\sigma_0 = \min\{\phi_{\max}, \sigma\}$. Similarly, one can calculate the conditional mean protrusion length

$$\lambda_{\mathrm{hit}} = \frac{1}{\rho_{\mathrm{DT}}}\left[\frac{1}{\sigma}\int_0^{\sigma_0}\zeta(y)e^{-\zeta(y)/l}dy\right], \quad \text{(S1.5)}$$

and

$$\lambda_{\mathrm{miss}} = \frac{1}{1-\rho_{\mathrm{DT}}}\left[l - \frac{\sigma_0}{\sigma}(\zeta(\sigma_0)+l)e^{-\zeta(\sigma_0)/l} - \frac{1}{\sigma l}\int_d^{\zeta(\sigma_0)} xe^{-x/l}\zeta^{-1}(x)dx\right]. \quad \text{(S1.6)}$$

### B. Annulus-shaped target

Similarly, we compute the same quantities for the annulus-shaped target. The major difference is that the target distance is always $d_s$ for any $\Theta$, which yields

$$F_Z(x) = \mathbb{I}_{[d_s,\infty)}(x). \quad \text{(S1.7)}$$

Similar to the previous section, we have

$$\rho_{\mathrm{DT}} = e^{-d_s/l}, \quad \text{(S1.8)}$$

and

$$\lambda_{\mathrm{hit}} = d_s, \qquad \lambda_{\mathrm{miss}} = l - \frac{d_s}{e^{d_s/l}-1}. \quad \text{(S1.9)}$$

### C. Error estimation

We calculate the relative difference of $\rho_{\mathrm{DT}}^{-1}$ and $\lambda_{\mathrm{hit}}$ between the disk-shaped domain $\omega$ and the "polar rectangle" $\widehat{\Omega}$. It can make a contact to $\widehat{\Omega}$ by a single protrusion if $\Theta \in [-\sigma_0, \sigma_0]$ and $L \ge d$, which gives

$$\rho_{\mathrm{DT}}(\widehat{\Omega}) = \frac{\sigma_0}{\sigma}e^{-d/l}. \quad \text{(S1.10)}$$

Using Eq. (S1.4) yields

$$\frac{\delta[\rho_{\mathrm{DT}}^{-1}]}{\rho_{\mathrm{DT}}^{-1}} = 1 - \frac{1}{\sigma_0}\int_0^{\sigma_0} e^{-(\zeta(y)-d)/l}dy. \quad \text{(S1.11)}$$

Since

$$\zeta(y) < r + d, \quad \text{(S1.12)}$$

we have

$$\frac{1}{\sigma_0}\int_0^{\sigma_0} e^{-(\zeta(y)-d)/l}dy \ge e^{-r/l}.$$

Substituting this inequality into Eq. (S1.11) gives

$$\frac{\delta[\rho_{\mathrm{DT}}^{-1}]}{\rho_{\mathrm{DT}}^{-1}} \le 1 - e^{-r/l}. \quad \text{(S1.13)}$$

Another application of Eq. (S1.12) gives

$$\lambda_{\mathrm{DT}}(\Omega) < r + d. \quad \text{(S1.14)}$$

Together with the fact that $\lambda_{\mathrm{hit}}(\widehat{\Omega}) = d$, we finally have

$$\frac{\delta[\lambda_{\mathrm{hit}}]}{\lambda_{\mathrm{hit}}} = 1 - \frac{\lambda_{\mathrm{hit}}(\widehat{\Omega})}{\lambda_{\mathrm{hit}}(\Omega)} \le \frac{r}{r+d}. \quad \text{(S1.15)}$$

* h6kim@sas.upenn.edu

## S2. DIFFUSIVE TRANSPORT TO IDEALIZED TARGETS

In this section, we present the computation for the Laplace transform of the non-dimensionalized flux to the two idealized targets discussed in Sect. III.

### A. Disk-shaped target

First, we consider the disk which is centered at the origin with radius $r_0 = r/d$. Then one can naturally set the source location $x_{s,0} = (R_0, 0)$ where $R_0 = 1+r_0$. One interesting observation is that the total concentration flux only depends on the distance to the source

$$J_{\text{diff},0}\Big(t_0; x_{s,0}(y)\Big) \equiv J_{\text{diff},0}(t_0; R_0 - r_0),$$

where $x_{s,0}(y)$ is the source location parameterized by the arc length over the circle with radius $R_0$ and $x_{s,0}(0) = (R_0, 0)$. In order to use this symmetry, we introduce the averaged concentration

$$\bar{u}(x_0, t_0) = \frac{1}{2\pi R_0}\int_0^{2\pi R_0} u_0(x_0, t_0; x_{s,0}(y))dy.$$

Averaging the non-dimensionalized model equation (Eq. (III.1)) gives

$$\frac{\partial \bar{u}}{\partial t_0} = \nabla^2 \bar{u} - g_0\bar{u} + \frac{1}{2\pi R_0}\int_0^{2\pi R_0} \delta(x_0 - x_{s,0}(y))dy. \tag{S2.1}$$

Multiplying the smooth test function and performing integration by parts, one can show that it is equivalent to solve the equation in the polar coordinate

$$\frac{\partial \bar{u}}{\partial t_0} = \frac{1}{r}\frac{\partial}{\partial r}\left(r\frac{\partial \bar{u}}{\partial r}\right) - g_0\bar{u}, \tag{S2.2}$$

together with the boundary conditions

$$\bar{u}(r_0, t_0) = 0, \qquad \lim_{r\to\infty} \bar{u}(r, t_0) = 0, \tag{S2.3}$$

the jump condition induced from the delta function

$$[\bar{u}]_-^+ = 0, \qquad \left[\frac{\partial \bar{u}}{\partial r}\right]_-^+ = -\frac{1}{2\pi R_0}, \tag{S2.4}$$

where $[f(r)]_-^+ = \lim_{r\to R_0^+} f(r) - \lim_{r\to R_0^-} f(r)$. Taking the Laplace transform gives

$$s\mathcal{L}[\bar{u}](r,s) = \frac{1}{r}\frac{\partial}{\partial r}\left(r\frac{\partial \mathcal{L}[\bar{u}]}{\partial r}\right) - g_0\mathcal{L}[\bar{u}], \tag{S2.5}$$

whose general solution takes the form of

$$\mathcal{L}[\bar{u}](r,s) = A(s)I_0(r\sqrt{s+g_0}) + B(s)K_0(r\sqrt{s+g_0}),$$

where $I_\beta, K_\beta$ are the modified Bessel functions of the first and the second kind with order $\beta$, respectively. Matching the coefficients with the conditions

$$\mathcal{L}[\bar{u}](r_0, s) = 0, \qquad \lim_{r\to\infty} \mathcal{L}[\bar{u}](r,s) = 0, \tag{S2.6a}$$

$$\Big[\mathcal{L}[\bar{u}]\Big]_-^+ = 0, \qquad \left[\frac{\partial \mathcal{L}[\bar{u}]}{\partial r}\right]_-^+ = -\frac{1}{2\pi R_0 s}, \tag{S2.6b}$$

one can determine the solution

$$\mathcal{L}[\bar{u}](r,s) = \\ = \begin{cases} A_-(s)I_0(r\sqrt{s+g_0}) + B_-(s)K_0(r\sqrt{s+g_0}), & r \le R_0 \\ B_+(s)K_0(r\sqrt{s+g_0}), & r > R_0 \end{cases}$$

where

$$\begin{aligned} A_-(s) &= K_0(r_0\sqrt{s+g_0})Q(s) \\ B_-(s) &= -I_0(r_0\sqrt{s+g_0})Q(s) \\ B_+(s) &= A_-(s)I_0(R_0\sqrt{s+g_0})/K_0(R_0\sqrt{s+g_0}) + B_-(s) \end{aligned}$$

and

$$Q(s) = \frac{K_0(R_0\sqrt{s+g_0})}{2\pi s K_0(r_0\sqrt{s+g_0})}.$$

Then the Laplace transformation of the flux is

$$\begin{aligned} \mathcal{L}[J_{\text{diff},0}](s) &= 2\pi r_0 \left.\frac{\partial \mathcal{L}[\bar{u}]}{\partial r}\right|_{r=r_0} \\ &= \frac{K_0(R_0\sqrt{s+g_0})}{sK_0(r_0\sqrt{s+g_0})}. \end{aligned} \tag{S2.7}$$

This yields

$$\begin{aligned} J^{\text{ss}}_{\text{diff},0} &= \lim_{s\to 0} s\mathcal{L}[J_{\text{diff},0}](s) \\ &= \frac{K_0(R_0\sqrt{g_0})}{K_0(r_0\sqrt{g_0})}. \end{aligned} \tag{S2.8}$$

Moreover, the coefficient in the asymptotic equation (Eq. (III.8))

$$\overline{\psi}_{\text{diff},0}(V_0) = \frac{V_0}{\rho_{\text{diff}}} + \frac{1}{2}\Psi_{\text{diff}},$$

can be determined as follows:

$$\begin{aligned} \Psi_{\text{diff}} &= 2\lim_{s\to 0} \frac{1}{s} - \frac{\mathcal{L}[J_{\text{diff},0}](s)}{\rho_{\text{diff}}} \\ &= \mathcal{F}_K(1+r_0, g_0) - \mathcal{F}_K(r_0, g_0), \end{aligned} \tag{S2.9}$$

where $\mathcal{F}_K(x,y) = xK_1(x\sqrt{y})/(\sqrt{y}K_0(x\sqrt{y}))$.

### B. Annulus-shaped target

Next, we solve the non-dimensional diffusion equation for the annulus-shaped target together with the source

located at the center. That is, the concentration dynamics is governed by

$$\frac{\partial u_0}{\partial t_0} = \nabla^2 u_0 - g_0 u_0 + \delta(x_0), \tag{S2.10}$$

which is supplemented by the absorbing boundary condition

$$u(|x_0| = 1, t_0) = 0. \tag{S2.11}$$

Using a test function argument, one can derive an equivalent equation without the delta function in the polar coordinate

$$\frac{\partial u_0}{\partial t_0} = \frac{1}{r}\frac{\partial}{\partial r}\left(r\frac{\partial u_0}{\partial r}\right) - g_0 u_0, \tag{S2.12}$$

together with the boundary conditions

$$\lim_{r\to 0} r\frac{\partial u_0(r,t_0)}{\partial r} = -\frac{1}{2\pi}, \qquad u_0(1,t_0) = 0. \tag{S2.13}$$

Taking the Laplace transform in time

$$s\mathcal{L}[u_0](r,s) = \frac{1}{r}\frac{\partial}{\partial r}\left(r\frac{\partial \mathcal{L}[u_0]}{\partial r}\right) - g_0\mathcal{L}[u_0]. \tag{S2.14}$$

Similar to the previous section, the general solutions takes the form

$$\mathcal{L}[u_0](r,s) = A(s)I_0(r\sqrt{s+g_0}) + B(s)K_0(r\sqrt{s+g_0}).$$

Determining the coefficients by matching boundary conditions

$$\lim_{r\to 0} r\frac{\partial \mathcal{L}[u_0](r,s)}{\partial r} = -\frac{1}{2\pi s}, \qquad \mathcal{L}[u_0](1,s) = 0, \tag{S2.15}$$

we have the Laplace transform of the non-dimensional flux

$$\mathcal{L}[J_{\text{diff},0}](s) = \frac{1}{sI_0(\sqrt{s+g_0})}. \tag{S2.16}$$

This gives the asymptotic flux

$$\begin{aligned} J^{\text{ss}}_{\text{diff},0} &= \lim_{s\to 0}\mathcal{L}[J_{\text{diff},0}](s) \\ &= \frac{1}{I_0(\sqrt{g_0})}. \end{aligned} \tag{S2.17}$$

Using this, one can also determine the coefficient in the asymptotic approximation

$$\begin{aligned} \Psi_{\text{diff}} &= 2\lim_{s\to 0}\frac{1}{s} - \frac{\mathcal{L}[J_{\text{diff},0}](s)}{\rho_{\text{diff}}} \\ &= \mathcal{F}_I(g_0), \end{aligned} \tag{S2.18}$$

where $\mathcal{F}_I(x) = I_1(\sqrt{x})/(\sqrt{x}I_0(\sqrt{x}))$.

## C. Degradation along protrusion

Here, we relax the assumption about diffusive transport along protrusion, and now molecules are degraded. We calculate the hitting probability that signaling molecules (diffusing along with the protrusion) hit the target before degradation. The hitting probability corresponds with $\rho_{\text{diff},1}$ in Sect. V because the particles diffuse along with the one-dimensional protrusion under degradation. Then we show that $\rho_{\text{diff},1} \geq \rho_{\text{diff},2}$ by using the basic properties of modified Bessel function.

Similar to Sect. III, we non-dimensionalize equation for the signaling molecule concentration dynamics over protrusion

$$\frac{\partial u_0}{\partial t_0} = \frac{\partial^2 u_0}{\partial x_0^2} - g_0 u_0, \quad 0 < x_0 < 1, \tag{S2.19}$$

together with the boundary condition

$$u_0(1,t_0) = 0, \quad \frac{\partial u_0}{\partial x_0} = -1. \tag{S2.20}$$

The steady-state solution takes the form

$$\lim_{t_0\to\infty} u_0(x_0,t_0) = \frac{\sinh\sqrt{g_0}(1-x_0)}{\sqrt{g_0}\cosh\sqrt{g_0}}. \tag{S2.21}$$

Taking spatial derivative yields the stationary flux at the target boundary, which is the same as the hitting probability of molecules before degradation

$$\rho_{\text{diff},1} = \frac{1}{\cosh\sqrt{g_0}}. \tag{S2.22}$$

Next, we show $\rho_{\text{diff},1} \geq \rho_{\text{diff}.2}$. We recall Eq. (S2.8), the hitting probability of mortal diffusive particles to the disk in 2D

$$\rho_{\text{diff},2} = \frac{K_0(R_0\sqrt{g_0})}{K_0(r_0\sqrt{g_0})}. \tag{S2.23}$$

$\rho_{\text{diff},1} - \rho_{\text{diff}.2}$ can be written by

$$G(x,y) = \frac{K_0(y) - \cosh(x)K_0(x+y)}{\cosh(x)K_0(y)},$$

by setting $\sqrt{g_0} = x$ and $r_0\sqrt{g_0} = y$. Since $\cosh(x) > 0$ and $K_0(y) > 0$ for $x,y > 0$, showing $G(x,y)$ is non-negative is equivalent to show that the numerator, $g(x,y) = K_0(y) - \cosh(x)K_0(x+y)$, is non-negative. Taking derivative with respect to $x$ and using the fact that $K_\beta < K_{\beta+1}$, we have

$$\begin{aligned} \frac{\partial g}{\partial x} &= \cosh(x)K_1(x+y) - \sinh(x)K_0(x,y) \\ &> [\cosh(x) - \sinh(x)]K_1(x+y) \\ &\geq 0. \end{aligned} \tag{S2.24}$$

Since $g(0,y) = 0$, we therefore proved the claim.

## S3. RARE-EVENT APPROXIMATION OF COST-BENEFIT RATIO

### A. Contact formation of direct transport model

The correlation of $\mathcal{X}$ and $\mathcal{T}_{\rm DT}$ can be analyzed under the rare-event approximation

$$\widetilde{\gamma}_{\rm DT} = \gamma_{0,\rm DT}^{-1}\mathbb{E}[\widetilde{\mathcal{X}}\widetilde{\mathcal{T}}_{\rm DT}]. \tag{S3.1}$$

Since $\mathcal{K}_0$ and $X_{{\rm hit},\mathcal{K}_0}$ are independent, one can condition the expectation value by setting $\mathcal{K}_0 = j$ and $X_{{\rm hit},\mathcal{K}_0} = x$

$$\begin{aligned}\frac{\widetilde{\gamma}_{{\rm DT},j}(x)}{\gamma_{0,\rm DT}^{-1}} &= \mathbb{E}[\widetilde{\mathcal{X}}\widetilde{\mathcal{T}}_{\rm DT}|\mathcal{K}_0 = j, X_{{\rm hit},\mathcal{K}_0} = x] \\ &= \frac{j\widetilde{\xi}_j}{\kappa_{\rm DT}} + \frac{(j-1)x\lambda_{\rm miss}}{v_+} + \frac{x^2}{v_+} \\ &\quad + \frac{x}{v_+}\mathbb{E}\left[\sum_{k=1}^{\mathcal{N}_0(x/v_+)} X_k\right].\end{aligned} \tag{S3.2}$$

Since we have

$$\mathbb{E}\left[\sum_{k=1}^{\mathcal{N}_0(x/v_+)} X_k\right] = \frac{\kappa_{\rm DT}x\lambda}{v_+}$$

then the cost-benefit ratio takes the form

$$\frac{\widetilde{\gamma}_{{\rm DT},j}(x)}{\gamma_{0,\rm DT}^{-1}} = \frac{j\widetilde{\xi}_j}{\kappa_{\rm DT}} + \frac{(j-1)x\lambda_{\rm miss}}{v_+} + \left(\frac{1}{v_+} + \frac{\kappa_{\rm DT}\lambda}{v_+^2}\right)x^2. \tag{S3.3}$$

Taking expectation with respect to $x = X_{\rm hit}$

$$\begin{aligned}\frac{\widetilde{\gamma}_{{\rm DT},j}}{\gamma_{0,\rm DT}^{-1}} &= \frac{\mathbb{E}[\widetilde{\gamma}_{{\rm DT},j}(X_{\rm hit})]}{\gamma_{0,\rm DT}^{-1}} \\ &= \frac{j\widetilde{\xi}_j}{\kappa_{\rm DT}} + (j-1)\tau_{\rm hit}\lambda_{\rm miss} \\ &\quad + \left(\frac{1}{v_+} + \frac{\kappa_{\rm DT}\lambda}{v_+^2}\right)\mathbb{E}[X_{\rm hit}^2].\end{aligned} \tag{S3.4}$$

Another application of the total expectation theorem gives the rare-event approximation of the cost-benefit ratio

$$\begin{aligned}\frac{\widetilde{\gamma}_{\rm DT}}{\gamma_{0,\rm DT}^{-1}} &= \mathbb{E}\left[\mathbb{E}[\widetilde{\mathcal{X}}\widetilde{\mathcal{T}}_{\rm DT}|\mathcal{K}_0, X_{{\rm hit},\mathcal{K}_0}]\right] \\ &= \widetilde{\tau}\widetilde{\xi} + \frac{\lambda_{\rm miss}}{\kappa_{\rm DT}}\frac{1-\rho_{\rm DT}}{\rho_{\rm DT}^2} \\ &\quad + (v_+ + \kappa_{\rm DT}\lambda)\,{\rm Var}[T_{\rm hit}^2],\end{aligned} \tag{S3.5}$$

where ${\rm Var}[T_{\rm hit}]$ is the variance of $T_{\rm hit}$. This also can be expanded as a power series of $\kappa_{\rm DT}$

$$\frac{\widetilde{\gamma}_{\rm DT}}{\gamma_{0,\rm DT}^{-1}} = \frac{c_{-1}}{\rho_{\rm DT}^2\kappa_{\rm DT}} + c_1\lambda\kappa_{\rm DT} + c_0, \tag{S3.6}$$

where $c_{-1} = \lambda + (1-\rho_{\rm DT})\lambda_{\rm miss}$, $c_1 = \mathbb{E}[T_{\rm hit}^2]$, and $c_0 = v_+{\rm Var}[T_{\rm hit}] + 2\tau_{\rm hit}\lambda/\rho_{\rm DT}$.

### B. Direct transport model with molecule transport

Similar to the previous section, we have the rare-event approximation of the cost-benefit ratio

$$\begin{aligned}\frac{\widetilde{\gamma}_{\Sigma,\rm DT}}{\gamma_0^{-1}} &= \mathbb{E}\Big[\big(\widetilde{\mathcal{T}}_{\rm DT} + \Psi_{\rm DT}(V;X_{\rm hit})\big)\big(\Delta_{\rm DT}\widetilde{\mathcal{X}} + \Delta_p V\big)\Big] \\ &= \widetilde{\gamma}_{\rm DT} + \Delta_p V\left(\widetilde{\tau}_{\rm DT} + \psi_{\rm DT}^{(0)}(V)\right) \\ &\quad + \Delta_{\rm DT}\mathbb{E}[\widetilde{\mathcal{X}}\Psi_{\rm DT}(V;X_{\rm hit})],\end{aligned} \tag{S3.7}$$

where $\psi_{\rm DT}^{(k)}(V) = \mathbb{E}[X_{\rm hit}^k\Psi_{\rm DT}(V;X_{\rm hit})]$ for $k = 0, 1, \cdots$. Since $\widetilde{\mathcal{X}}$ also contains $X_{\rm hit}$, the last term is deduced to with the higher-order moment term

$$\begin{aligned}&\mathbb{E}[\widetilde{\mathcal{X}}\Psi_{\rm DT}(V;X_{\rm hit})] \\ &\quad = \frac{1-\rho_{\rm DT}}{\rho_{\rm DT}}\lambda_{\rm miss}\psi_{\rm DT}^{(0)}(V) + \frac{1}{v_+}(v_+ + \kappa_{\rm DT}\lambda)\psi_{\rm DT}^{(1)}(V).\end{aligned} \tag{S3.8}$$

This approximation can be written as a power series of $\kappa_{\rm DT}$

$$\frac{\widetilde{\gamma}_{\Sigma,\rm DT}}{\gamma_{0,\rm DT}^{-1}} - \frac{\widetilde{\gamma}_{\rm DT}}{\gamma_{0,\rm DT}^{-1}} = c_{\Sigma,-1}\Delta_p V\kappa_{\rm DT}^{-1} + c_{\Sigma,1}\psi_{\rm DT}^{(1)}(V)\kappa_{\rm DT} + c_{\Sigma,0}. \tag{S3.9}$$

where $c_{\Sigma,-1} = \Delta_{\rm DT}^{-1}\rho_{\rm DT}^{-1}$, $c_{\Sigma,1} = \lambda/v_+$, and $c_{\Sigma,0} = (1-\rho_{\rm DT})\lambda_{\rm miss}\psi_{\rm DT}^{(0)}(V)/\rho_{\rm DT} + \Delta_p V\psi_{\rm DT}^{(0)}(V)/\Delta_{\rm DT} + \psi_{\rm DT}^{(1)}(V)$.

### C. Total energetic cost

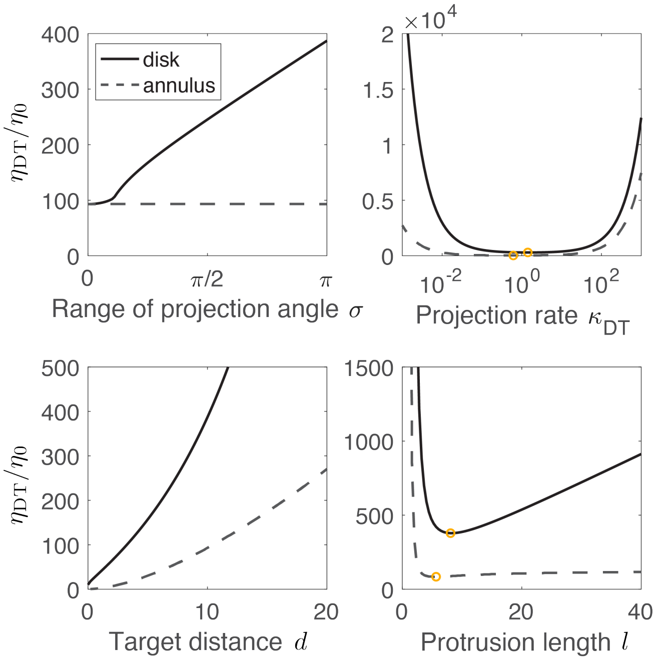


FIG. S1. Corresponding plot of Fig. 8 in case of the total energetic cost. Parameters are chosen as follows: $\Delta_{\rm DT}/\eta_0 = 1\,{\rm min}/\mu{\rm m}$ and the others are the same as Fig. 8.

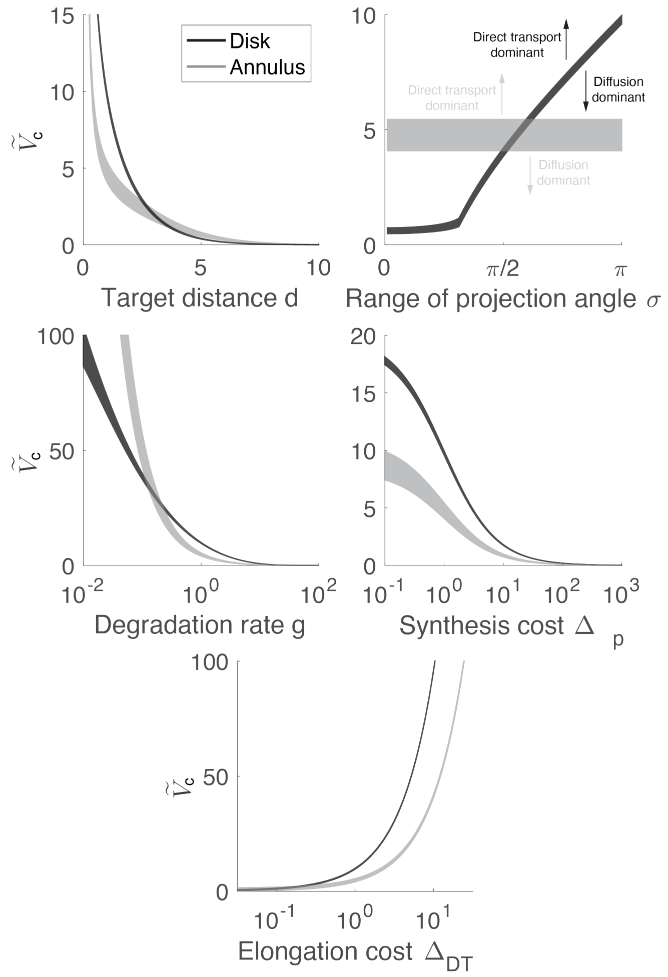


FIG. S2. Corresponding plot of Fig. 11 in case of the total energetic cost. Parameters are chosen as follows: $\eta_0 = 1\varepsilon/\min$ and the others are the same as Fig. 11.
